# Supplementary material for: Restoring Images in Adverse Weather Conditions via Histogram Transformer
Source: arXiv:2407.10172 source file (2024-07-25)
Supplement: Supplementary file 2 [file supple_rainfog-1.tex]

\begin{figure*}
  \centering
  \begin{minipage}{0.330\linewidth}
    \centering
  \begin{subfigure}{1\linewidth}
    \includegraphics[width=1\linewidth]{fig/result/rainfog/rect/input_im_0343_s95_a05.png}
  \end{subfigure}
  \hspace{-1.5mm}
  \begin{subfigure}{0.493\linewidth}
    \includegraphics[width=1\linewidth]{fig/result/rainfog/rect/input_patch0_im_0343_s95_a05.png}
  \end{subfigure}
  \hspace{-1.5mm}
  \begin{subfigure}{0.493\linewidth}
    \includegraphics[width=1\linewidth]{fig/result/rainfog/rect/input_patch1_im_0343_s95_a05.png}
  \end{subfigure}
    \subcaption[]{Input}
    \end{minipage}
  \hspace{-1.5mm}
  \begin{minipage}{0.330\linewidth}
    \centering
  \begin{subfigure}{1\linewidth}
    \includegraphics[width=1\linewidth]{fig/result/rainfog/rect/mprnet_im_0343_s95_a05.png}
  \end{subfigure}
  \hspace{-1.5mm}
  \begin{subfigure}{0.493\linewidth}
    \includegraphics[width=1\linewidth]{fig/result/rainfog/rect/mprnet_patch0_im_0343_s95_a05.png}
  \end{subfigure}
  \hspace{-1.5mm}
  \begin{subfigure}{0.493\linewidth}
    \includegraphics[width=1\linewidth]{fig/result/rainfog/rect/mprnet_patch1_im_0343_s95_a05.png}
  \end{subfigure}
    \subcaption[]{MPRNet~\cite{Zamir2021mprnet}}
    \end{minipage}
  \hspace{-1.5mm}
  \begin{minipage}{0.330\linewidth}
    \centering
  \begin{subfigure}{1\linewidth}
    \includegraphics[width=1\linewidth]{fig/result/rainfog/rect/restormer_im_0343_s95_a05.png}
  \end{subfigure}
  \hspace{-1.5mm}
  \begin{subfigure}{0.493\linewidth}
    \includegraphics[width=1\linewidth]{fig/result/rainfog/rect/restormer_patch0_im_0343_s95_a05.png}
  \end{subfigure}
  \hspace{-1.5mm}
  \begin{subfigure}{0.493\linewidth}
    \includegraphics[width=1\linewidth]{fig/result/rainfog/rect/restormer_patch1_im_0343_s95_a05.png}
  \end{subfigure}
    \subcaption[]{Restormer~\cite{zamir2022restormer}}
    \end{minipage}
  \hspace{-1.5mm}
  \begin{minipage}{0.330\linewidth}
    \centering
  \begin{subfigure}{1\linewidth}
    \includegraphics[width=1\linewidth]{fig/result/rainfog/rect/transweather_im_0343_s95_a05.png}
  \end{subfigure}
  \hspace{-1.5mm}
  \begin{subfigure}{0.493\linewidth}
    \includegraphics[width=1\linewidth]{fig/result/rainfog/rect/transweather_patch0_im_0343_s95_a05.png}
  \end{subfigure}
  \hspace{-1.5mm}
  \begin{subfigure}{0.493\linewidth}
    \includegraphics[width=1\linewidth]{fig/result/rainfog/rect/transweather_patch1_im_0343_s95_a05.png}
  \end{subfigure}
    \subcaption[]{TransWeather~\cite{valanarasu2022transweather}}
    \end{minipage}
  \hspace{-1.5mm}
  \begin{minipage}{0.330\linewidth}
    \centering
  \begin{subfigure}{1\linewidth}
    \includegraphics[width=1\linewidth]{fig/result/rainfog/rect/chen_im_0343_s95_a05.png}
  \end{subfigure}
  \hspace{-1.5mm}
  \begin{subfigure}{0.493\linewidth}
    \includegraphics[width=1\linewidth]{fig/result/rainfog/rect/chen_patch0_im_0343_s95_a05.png}
  \end{subfigure}
  \hspace{-1.5mm}
  \begin{subfigure}{0.493\linewidth}
    \includegraphics[width=1\linewidth]{fig/result/rainfog/rect/chen_patch1_im_0343_s95_a05.png}
  \end{subfigure}
    \subcaption[]{Chen \textit{et al}.~\cite{Chen2022MultiWeatherRemoval}}
    \end{minipage}
  \hspace{-1.5mm}
  \begin{minipage}{0.330\linewidth}
    \centering
  \begin{subfigure}{1\linewidth}
    \includegraphics[width=1\linewidth]{fig/result/rainfog/rect/wgws_im_0343_s95_a05.png}
  \end{subfigure}
  \hspace{-1.5mm}
  \begin{subfigure}{0.493\linewidth}
    \includegraphics[width=1\linewidth]{fig/result/rainfog/rect/wgws_patch0_im_0343_s95_a05.png}
  \end{subfigure}
  \hspace{-1.5mm}
  \begin{subfigure}{0.493\linewidth}
    \includegraphics[width=1\linewidth]{fig/result/rainfog/rect/wgws_patch1_im_0343_s95_a05.png}
  \end{subfigure}
    \subcaption[]{WGWS-Net~\cite{zhu2023learning_wgwsnet}}
    \end{minipage}
  \hspace{-1.5mm}
  \begin{minipage}{0.330\linewidth}
    \centering
  \begin{subfigure}{1\linewidth}
    \includegraphics[width=1\linewidth]{fig/result/rainfog/rect/weatherdiff_im_0343_s95_a05.jpg}
  \end{subfigure}
  \hspace{-1.5mm}
  \begin{subfigure}{0.493\linewidth}
    \includegraphics[width=1\linewidth]{fig/result/rainfog/rect/weatherdiff_patch0_im_0343_s95_a05.jpg}
  \end{subfigure}
  \hspace{-1.5mm}
  \begin{subfigure}{0.493\linewidth}
    \includegraphics[width=1\linewidth]{fig/result/rainfog/rect/weatherdiff_patch1_im_0343_s95_a05.jpg}
  \end{subfigure}
    \subcaption[]{WeatherDiff$_{64}$~\cite{ozdenizci2023restoring}}
    \end{minipage}
  \hspace{-1.5mm}
  \begin{minipage}{0.330\linewidth}
    \centering
  \begin{subfigure}{1\linewidth}
    \includegraphics[width=1\linewidth]{fig/result/rainfog/rect/histoformer_im_0343_s95_a05.png}
  \end{subfigure}
  \hspace{-1.5mm}
  \begin{subfigure}{0.493\linewidth}
    \includegraphics[width=1\linewidth]{fig/result/rainfog/rect/histoformer_patch0_im_0343_s95_a05.png}
  \end{subfigure}
  \hspace{-1.5mm}
  \begin{subfigure}{0.493\linewidth}
    \includegraphics[width=1\linewidth]{fig/result/rainfog/rect/histoformer_patch1_im_0343_s95_a05.png}
  \end{subfigure}
    \subcaption[]{Ours}
    \end{minipage}
  \hspace{-1.5mm}
  \begin{minipage}{0.330\linewidth}
    \centering
  \begin{subfigure}{1\linewidth}
    \includegraphics[width=1\linewidth]{fig/result/rainfog/rect/gt_im_0343_s95_a05.png}
  \end{subfigure}
  \hspace{-1.5mm}
  \begin{subfigure}{0.493\linewidth}
    \includegraphics[width=1\linewidth]{fig/result/rainfog/rect/gt_patch0_im_0343_s95_a05.png}
  \end{subfigure}
  \hspace{-1.5mm}
  \begin{subfigure}{0.493\linewidth}
    \includegraphics[width=1\linewidth]{fig/result/rainfog/rect/gt_patch1_im_0343_s95_a05.png}
  \end{subfigure}
    \subcaption[]{Ground-truth}
    \end{minipage}
  \caption{A visual comparison of rain streak and haze removal on Outdoor-Rain~\cite{li2019heavy}.}
  \label{fig:rainfog-supple-1}
\end{figure*}
