# Supplementary material for: Restoring Images in Adverse Weather Conditions via Histogram Transformer
Source: arXiv:2407.10172 source file (2024-07-25)
Supplement: Supplementary file 4 [file supple_snow-1.tex]

\begin{figure*}
  \centering
  \begin{minipage}{0.330\linewidth}
    \centering
  \begin{subfigure}{1\linewidth}
    \includegraphics[width=1\linewidth]{fig/result/snow/rect/input_winter_weather_05086.jpg}
  \end{subfigure}
  \hspace{-1.5mm}
  \begin{subfigure}{0.493\linewidth}
    \includegraphics[width=1\linewidth]{fig/result/snow/rect/input_patch0_winter_weather_05086.jpg}
  \end{subfigure}
  \hspace{-1.5mm}
  \begin{subfigure}{0.493\linewidth}
    \includegraphics[width=1\linewidth]{fig/result/snow/rect/input_patch1_winter_weather_05086.jpg}
  \end{subfigure}
    \subcaption[]{Input}
    \end{minipage}
  \hspace{-1.5mm}
  \begin{minipage}{0.330\linewidth}
    \centering
  \begin{subfigure}{1\linewidth}
    \includegraphics[width=1\linewidth]{fig/result/snow/rect/ddmsnet_winter_weather_05086.png}
  \end{subfigure}
  \hspace{-1.5mm}
  \begin{subfigure}{0.493\linewidth}
    \includegraphics[width=1\linewidth]{fig/result/snow/rect/ddmsnet_patch0_winter_weather_05086.png}
  \end{subfigure}
  \hspace{-1.5mm}
  \begin{subfigure}{0.493\linewidth}
    \includegraphics[width=1\linewidth]{fig/result/snow/rect/ddmsnet_patch1_winter_weather_05086.png}
  \end{subfigure}
    \subcaption[]{DDMSNet~\cite{zhang2021deep}}
    \end{minipage}
  \hspace{-1.5mm}
  \begin{minipage}{0.330\linewidth}
    \centering
  \begin{subfigure}{1\linewidth}
    \includegraphics[width=1\linewidth]{fig/result/snow/rect/restormer_winter_weather_05086.jpg}
  \end{subfigure}
  \hspace{-1.5mm}
  \begin{subfigure}{0.493\linewidth}
    \includegraphics[width=1\linewidth]{fig/result/snow/rect/restormer_patch0_winter_weather_05086.jpg}
  \end{subfigure}
  \hspace{-1.5mm}
  \begin{subfigure}{0.493\linewidth}
    \includegraphics[width=1\linewidth]{fig/result/snow/rect/restormer_patch1_winter_weather_05086.jpg}
  \end{subfigure}
    \subcaption[]{Restormer~\cite{zamir2022restormer}}
    \end{minipage}
  \hspace{-1.5mm}
  \begin{minipage}{0.330\linewidth}
    \centering
  \begin{subfigure}{1\linewidth}
    \includegraphics[width=1\linewidth]{fig/result/snow/rect/transweather_winter_weather_05086.jpg}
  \end{subfigure}
  \hspace{-1.5mm}
  \begin{subfigure}{0.493\linewidth}
    \includegraphics[width=1\linewidth]{fig/result/snow/rect/transweather_patch0_winter_weather_05086.jpg}
  \end{subfigure}
  \hspace{-1.5mm}
  \begin{subfigure}{0.493\linewidth}
    \includegraphics[width=1\linewidth]{fig/result/snow/rect/transweather_patch1_winter_weather_05086.jpg}
  \end{subfigure}
    \subcaption[]{TransWeather~\cite{valanarasu2022transweather}}
    \end{minipage}
  \hspace{-1.5mm}
  \begin{minipage}{0.330\linewidth}
    \centering
  \begin{subfigure}{1\linewidth}
    \includegraphics[width=1\linewidth]{fig/result/snow/rect/chen_winter_weather_05086.jpg}
  \end{subfigure}
  \hspace{-1.5mm}
  \begin{subfigure}{0.493\linewidth}
    \includegraphics[width=1\linewidth]{fig/result/snow/rect/chen_patch0_winter_weather_05086.jpg}
  \end{subfigure}
  \hspace{-1.5mm}
  \begin{subfigure}{0.493\linewidth}
    \includegraphics[width=1\linewidth]{fig/result/snow/rect/chen_patch1_winter_weather_05086.jpg}
  \end{subfigure}
    \subcaption[]{Chen \textit{et al}.~\cite{Chen2022MultiWeatherRemoval}}
    \end{minipage}
  \hspace{-1.5mm}
  \begin{minipage}{0.330\linewidth}
    \centering
  \begin{subfigure}{1\linewidth}
    \includegraphics[width=1\linewidth]{fig/result/snow/rect/wgws_winter_weather_05086.jpg}
  \end{subfigure}
  \hspace{-1.5mm}
  \begin{subfigure}{0.493\linewidth}
    \includegraphics[width=1\linewidth]{fig/result/snow/rect/wgws_patch0_winter_weather_05086.jpg}
  \end{subfigure}
  \hspace{-1.5mm}
  \begin{subfigure}{0.493\linewidth}
    \includegraphics[width=1\linewidth]{fig/result/snow/rect/wgws_patch1_winter_weather_05086.jpg}
  \end{subfigure}
    \subcaption[]{WGWS-Net~\cite{zhu2023learning_wgwsnet}}
    \end{minipage}
  \hspace{-1.5mm}
  \begin{minipage}{0.330\linewidth}
    \centering
  \begin{subfigure}{1\linewidth}
    \includegraphics[width=1\linewidth]{fig/result/snow/rect/weatherdiff_winter_weather_05086.jpg}
  \end{subfigure}
  \hspace{-1.5mm}
  \begin{subfigure}{0.493\linewidth}
    \includegraphics[width=1\linewidth]{fig/result/snow/rect/weatherdiff_patch0_winter_weather_05086.jpg}
  \end{subfigure}
  \hspace{-1.5mm}
  \begin{subfigure}{0.493\linewidth}
    \includegraphics[width=1\linewidth]{fig/result/snow/rect/weatherdiff_patch1_winter_weather_05086.jpg}
  \end{subfigure}
    \subcaption[]{WeatherDiff$_{64}$~\cite{ozdenizci2023restoring}}
    \end{minipage}
  \hspace{-1.5mm}
  \begin{minipage}{0.330\linewidth}
    \centering
  \begin{subfigure}{1\linewidth}
    \includegraphics[width=1\linewidth]{fig/result/snow/rect/histoformer_winter_weather_05086.png}
  \end{subfigure}
  \hspace{-1.5mm}
  \begin{subfigure}{0.493\linewidth}
    \includegraphics[width=1\linewidth]{fig/result/snow/rect/histoformer_patch0_winter_weather_05086.png}
  \end{subfigure}
  \hspace{-1.5mm}
  \begin{subfigure}{0.493\linewidth}
    \includegraphics[width=1\linewidth]{fig/result/snow/rect/histoformer_patch1_winter_weather_05086.png}
  \end{subfigure}
    \subcaption[]{Ours}
    \end{minipage}
  \hspace{-1.5mm}
  \begin{minipage}{0.330\linewidth}
    \centering
  \begin{subfigure}{1\linewidth}
    \includegraphics[width=1\linewidth]{fig/result/snow/rect/gt_winter_weather_05086.jpg}
  \end{subfigure}
  \hspace{-1.5mm}
  \begin{subfigure}{0.493\linewidth}
    \includegraphics[width=1\linewidth]{fig/result/snow/rect/gt_patch0_winter_weather_05086.jpg}
  \end{subfigure}
  \hspace{-1.5mm}
  \begin{subfigure}{0.493\linewidth}
    \includegraphics[width=1\linewidth]{fig/result/snow/rect/gt_patch1_winter_weather_05086.jpg}
  \end{subfigure}
    \subcaption[]{Ground-truth}
    \end{minipage}
  \caption{A visual comparisons of desnowing on Snow100K-L~\cite{liu2018desnownet}.}
  \label{fig:snow-supple-1}
\end{figure*}
