# Supplementary material for: Restoring Images in Adverse Weather Conditions via Histogram Transformer
Source: arXiv:2407.10172 source file (2024-07-25)
Supplement: Supplementary file 11 [file supple_realsnow-2.tex]

\begin{figure*}
\vspace{-5mm}
  \centering
  \begin{minipage}{0.455\linewidth}
    \centering
  \begin{subfigure}{1\linewidth}
    \includegraphics[width=1\linewidth]{fig/result/realsnow/input/first_snow_00416.jpg}
  \end{subfigure}
    \subcaption[]{Input}
    \end{minipage}
  \hspace{-1mm}
  \begin{minipage}{0.455\linewidth}
    \centering
  \begin{subfigure}{1\linewidth}
    \includegraphics[width=1\linewidth]{fig/result/realsnow/ddmsnet/first_snow_00416.png}
  \end{subfigure}
    \subcaption[]{DDMSNet~\cite{zhang2021deep}}
    \end{minipage}
  \hspace{-1mm}
  \begin{minipage}{0.455\linewidth}
    \centering
  \begin{subfigure}{1\linewidth}
    \includegraphics[width=1\linewidth]{fig/result/realsnow/restormer/first_snow_00416.jpg}
  \end{subfigure}
    \subcaption[]{Restormer~\cite{zamir2022restormer}}
    \end{minipage}
  \hspace{-1mm}
  \begin{minipage}{0.455\linewidth}
    \centering
  \begin{subfigure}{1\linewidth}
    \includegraphics[width=1\linewidth]{fig/result/realsnow/transweather/first_snow_00416.jpg}
  \end{subfigure}
    \subcaption[]{TransWeather~\cite{valanarasu2022transweather}}
    \end{minipage}
  \hspace{-1mm}
  \begin{minipage}{0.455\linewidth}
    \centering
  \begin{subfigure}{1\linewidth}
    \includegraphics[width=1\linewidth]{fig/result/realsnow/chen/first_snow_00416.jpg}
  \end{subfigure}
    \subcaption[]{Chen \textit{et al}.~\cite{Chen2022MultiWeatherRemoval}}
    \end{minipage}
  \hspace{-1mm}
  \begin{minipage}{0.455\linewidth}
    \centering
  \begin{subfigure}{1\linewidth}
    \includegraphics[width=1\linewidth]{fig/result/realsnow/wgws/first_snow_00416.jpg}
  \end{subfigure}
    \subcaption[]{WGWS-Net~\cite{zhu2023learning_wgwsnet}}
    \end{minipage}
  \hspace{-1mm}
  \begin{minipage}{0.455\linewidth}
    \centering
  \begin{subfigure}{1\linewidth}
    \includegraphics[width=1\linewidth]{fig/result/realsnow/weatherdiff/first_snow_00416.jpg}
  \end{subfigure}
    \subcaption[]{WeatherDiff$_{64}$~\cite{ozdenizci2023restoring}}
    \end{minipage}
  \hspace{-1mm}
  \begin{minipage}{0.455\linewidth}
    \centering
  \begin{subfigure}{1\linewidth}
    \includegraphics[width=1\linewidth]{fig/result/realsnow/histoformer/first_snow_00416.png}
  \end{subfigure}
    \subcaption[]{Ours}
    \end{minipage}
  \vspace{-3mm}
  \caption{A visual comparison of real-world desnowing on Snow100K~\cite{liu2018desnownet}.}
  \label{fig:realsnow-supple-2}
\end{figure*}
